# Supplementary material for: Unusual magnetotransport and anomalous Hall effect in quasi-two-dimensional van der Waals ferromagnet Fe$_4$GeTe$_2$
Source: arXiv:2303.07440 ancillary file (2023-03-13)
Supplement: Supplementary file 1 [file manuscript_supple.pdf]

# Supplementary Information

## Unusual magnetotransport and anomalous Hall effect in quasi-two-dimensional van der Waals ferromagnet $Fe_4GeTe_2$

Riju Pal[1], Buddhadeb Pal[1], Suchanda Mondal[2], Prabhat Mandal[1], and Atindra Nath Pal[1]

[1]Department of Condensed Matter Physics and Material Sciences, S. N. Bose National Centre for Basic Sciences, Block–JD, Sector–III, Salt Lake, Kolkata, 700106, India

[2]Saha Institute of Nuclear Physics, HBNI, 1/AF Bidhannagar, Calcutta 700064, India

## S1. Crystal preparation and characterization:

### S1.1 Crystal structure:

Single crystal $Fe_4GeTe_2$ is a van der Waals material with each single layer consists of seven atoms ($Fe_1$ and $Fe_2$ are arranged on both sides of the Ge atomic plane and directly connected with Te atoms), which forms a rhombohedral structure with space group $R\bar{3}m$ [1] (see Fig. 1.1). The thickness of monolayer $Fe_4GeTe_2$ is around 1 nm[1]. The extracted lattice parameters from the XRD analysis were found to be, a = 9.97Å and $\alpha = 23.3^0$, which are consistent with the reported value[1].

### S1.2 Sample preparation:

The single crystal $Fe_4GeTe_2$ was grown by the standard chemical vapor transport (CVT) method along with $I_2$ as a transport agent. Here, we have used the mixture of highly pure (99.99%) Fe, Ge and Te materials powder with a molar ratio 5: 1: 2 in a high vacuum quartz tube and this was heated for seven days at $725^0$ C. The resultant material was further inserted inside an evacuated quartz tube and placed in a gradient temperature based horizontal furnace with temperatures $800^0$ C and $750^0$ C maintained on both ends for seven days along with the transport agent $I_2$ (2 mg/cc), The details of the sample preparation are given in our earlier report[2]. The basic characterizations like X-ray diffraction (XRD) are performed on a cleaved thin and shiny single crystal of $Fe_4GeTe_2$. The presence of very sharp (0 0 l) peaks in the diffraction pattern confirms[2] that the flat plane of the crystal is perpendicular to the crystallographic c-axis with interlayer separation 28.74 Å. Also, high-resolution transmission electron microscopy (HRTEM), energy-dispersive X-ray (EDX) spectrum were performed[2], revealing good single crystal quality. Next, the magnetization measurements were done in a vibrating sample magnetometer (VSM) (DynaCool, Quantum Design) setup with magnetic field applied along both c-axis and in-plane directions.

**S1.3 Device fabrication:**

As these ferromagnetic materials are sensitive in ambient condition, we fabricated the Hall bar devices through dry transfer method on a prepatterned Ti (10 nm)/Au (45 nm) contacts on a 285 nm $SiO_2$/Si(p++) substrate. First, we fabricate gold pads using optical lithography and lift-off process followed by oxygen plasma treatment to clean the organic residues. Then we exfoliate thin layers of $Fe_4GeTe_2$ crystal by standard mechanical exfoliation on a thin PDMS layer and transferred on to the gold pads at an elevated temperature ($90^0$ C- $110^0$ C) using a home-made dry-transfer set up. The device was then immediately coated with PMMA to avoid any oxidation of the flake. Whole transfer process was completed within 30 minutes. The device was then bonded with silver paint (SPI supplies) and contacts are checked using SR830 lock-in and Keithley 2450 source-meter. All the contacts were found to be ohmic. The in-plane resistivity, Hall coefficient and other transport measurements are performed using standard lock-in techniques at frequency 234.1 Hz in a low-temperature magneto-transport setup (Teslatron, Oxford Instruments) in the temperature range: 1.6 K - 300 K. The four-terminal resistivity (ρ) is calculated from the measured resistance (R) using the formula, $\rho = R\times(W\times t/L)$, where W is the width of the flake, t is the thickness of the flake and L is distance between two longitudinal electrodes.

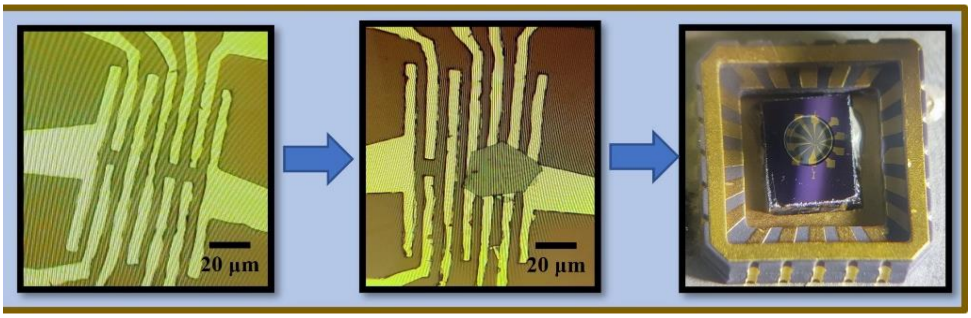


**Figure S1.3** Device fabrication procedures by dry transfer technique on a pre-patterned gold electrodes on Si/$SiO_2$ substrate.

**S1.4 Device characterization: Determination of the thickness via AFM**

Atomic force microscopy (AFM) was done to determine the thickness of the exfoliated $Fe_4GeTe_2$ crystal. After performing all the measurements, PMMA layer was removed from the top of the $Fe_4GeTe_2$ crystal and then AFM was performed immediately. The thickness of the exfoliated crystal is 95 nm (~ 95 layers), as determined from the height profile (Fig. S1.4).

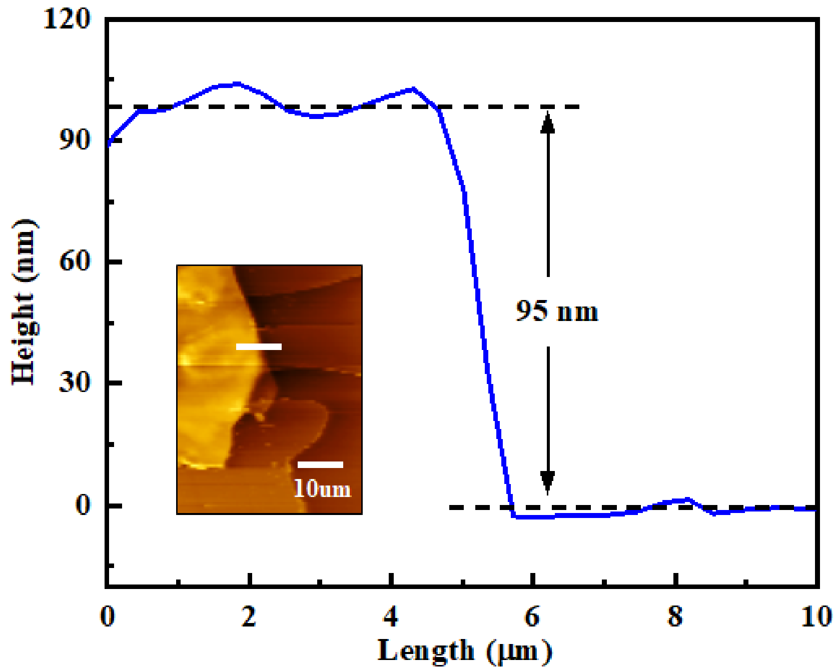


**Figure S1.4** Height profile of the $Fe_4GeTe_2$ flake on the Hall-bar device and corresponding AFM image. (inset)

## S2. Magnetic field dependent magnetization data: (M-B)

Magnetic field dependence of magnetization of the bulk $Fe_4GeTe_2$ sample is measured at different temperatures from 5 K to 300 K for B||c-axis and B||ab-plane is shown in Fig. S2 (a) and (c). The saturation magnetization ($M_S$) is calculated where the magnetic moment becomes almost independent on the applied magnetic fields. Above 7 T, M becomes saturated ($M_S$) from 5 K upto 100 K for both B||c-axis and B||ab-plane. But, above 120 K, there is a very weak dependency of the magnetization with the applied magnetic field. We have plotted $M_S$ (magnetization value above 7 T for B||c and B||ab plane) with temperature as in Fig. S2 (b) and (d). High field saturation magnetization value at 5 K is estimated to be about 1.9 $\mu_B$/Fe for both B||c-axis and B||ab-plane, consistent with the earlier reported value[1,2].

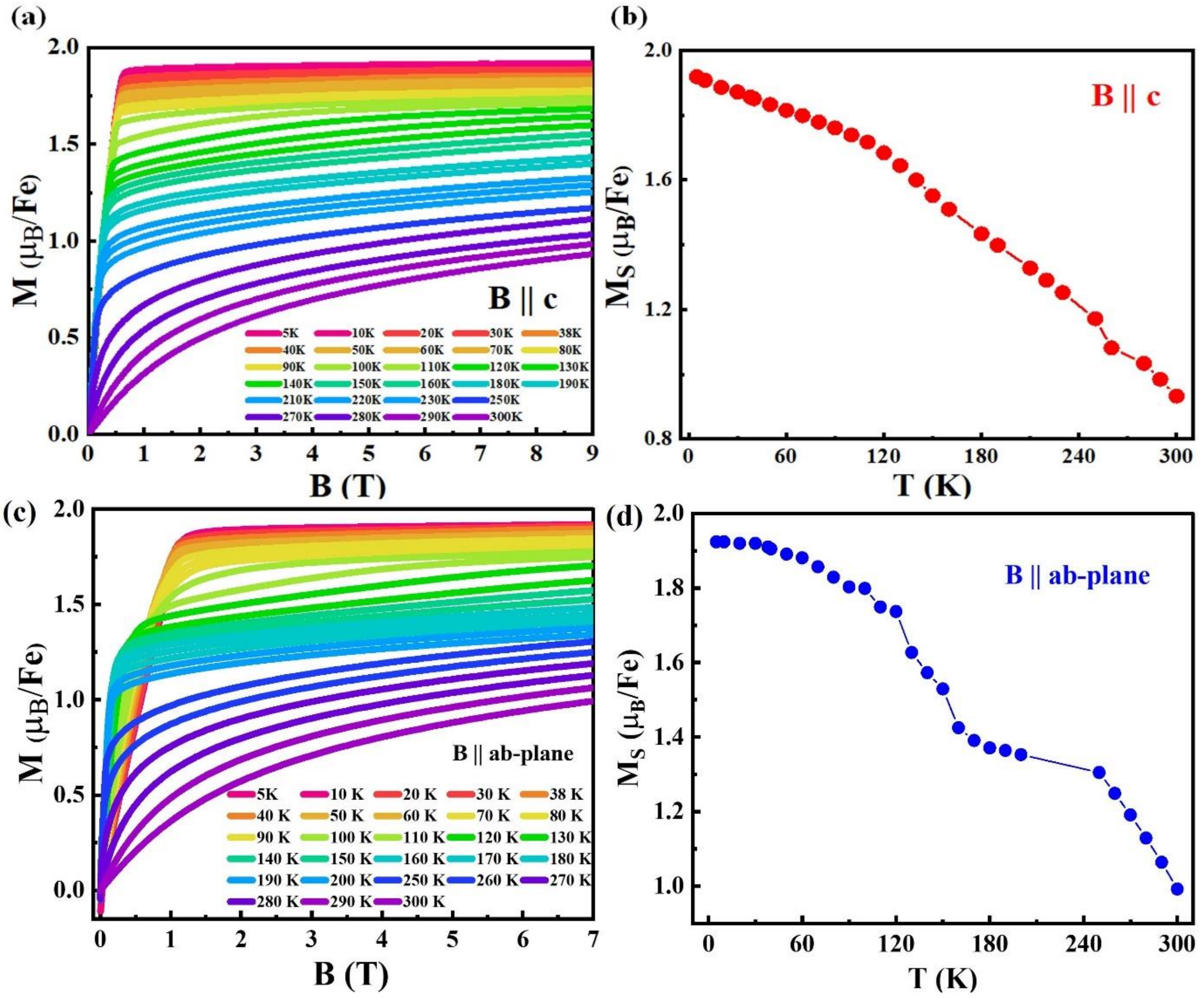


**Figure S2** Temperature dependence of magnetization data while magnetic field (B) is applied along c-axis **(a)** and along ab-plane **(c)**. Temperature dependence of the saturation magnetization ($M_S$) with B||c-axis **(b)** and B||ab-plane **(d)**.

## S3. Magnetic field dependence of R-T:

To decouple the scattering mechanisms, temperature and magnetic field dependence of resistance of another multilayer device was measured. The exact thickness of this flake was not measured, but the optical contrast suggests that the thickness could be in the range 30-50 nm and hence, the value of resistivity could not be determined. Fig. S3 (a) compares the R-T curves for magnetic field (9 T) applied both in-plane (IP) and out-of-plane (OP) direction of the crystal. We have fitted the resistivity data with ($T+T^2$) in the intermediate regime between 62 K - 122 K. From the fitting parameters, for zero field resistance data the coefficient of $T^2$ is $9.54 \times 10^{-4}$ Ω $K^{-2}$, but for 9 T in-plane and out-of-plane data this coefficient of $T^2$ reduces significantly to $2.56 \times 10^{-4}$ Ω $K^{-2}$ and $1.44 \times 10^{-4}$ Ω $K^{-2}$ respectively. This indicates that the electron-magnon scattering contribution is suppressed due to the application of higher magnetic field (9 T). This is more evident from the temperature derivative of the R-T data as shown in Fig. S3 (b). In the low temperature regime of 1.6 K - 38 K, the temperature dependence of resistance is almost insensitive to the magnetic field in both IP and OP direction, suggesting

that the scattering is dominated by the electron-electron scattering rather than the electron-magnon scattering as described in the main text.

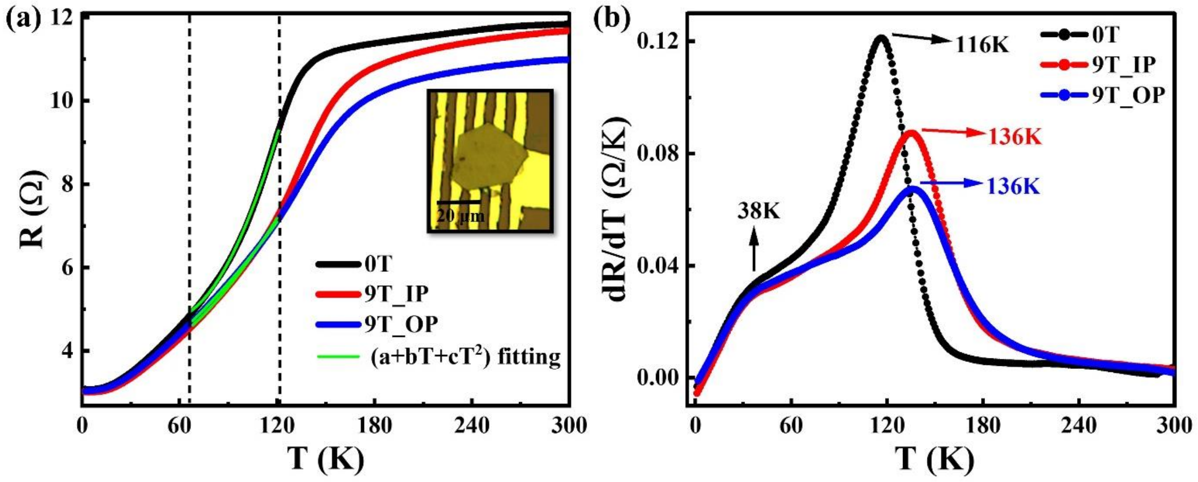


**Figure S3. (a)** Temperature dependence of resistance of the $Fe_4GeTe_2$ flake is measured at 0T and at magnetic field 9 T in both in-plane (IP) (red curve) and out-of-plane (OP) direction (blue curve). The data can be fitted with ($T+T^2$) in the range 62 K - 122 K, with the coefficient of $T^2$ decreasing with the magnetic field, which suggests a significant electron-magnon contribution in this temperature range. Inset: Optical micrograph of the multilayer flake on top of gold-electrodes on $Si/SiO_2$ substrate. **(b)** Temperature derivatives of the R-T curves show no magnetic field dependence up to 38 K, which supports electron-electron interaction below 38 K, however, with a strong magnetic field dependence in between 38 K - 240 K.

## S4. Additional analysis of magnetoresistance data:

### S4.1 Positive MR at low temperatures:

The orbital MR term in the total resistivity of a ferromagnetic material arises due to the constrained orbital motion by the free carriers under Lorentz force, which increases rapidly with the application of external magnetic field at low temperature. We have fitted low

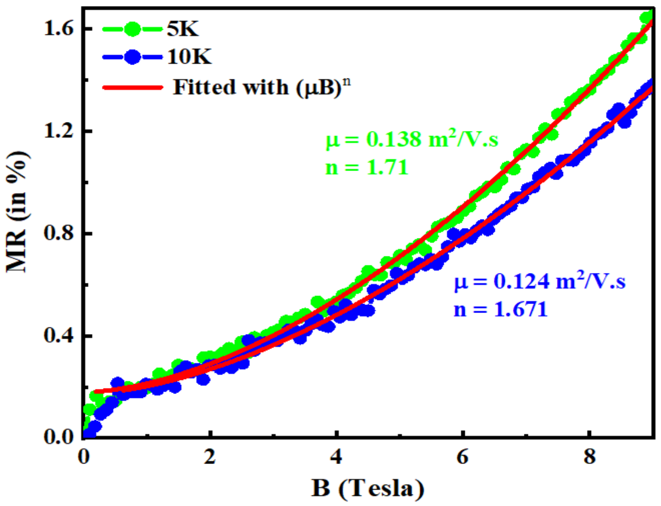


**Figure S4.1** Magnetic field dependent MR at 5 K and 10 K with B||c-axis and the corresponding fitting with the orbital MR term by the equation MR $\propto (\mu B)^n$ (Eq. 3)

temperature MR with Eq. (3) of the main text and obtained the parameters as follows: (i) For 1.6 K, μ = 0.147 $m^2$/V.s and n = 1.847 (See Fig.2(a) inset); (ii) For 5 K, μ = 0.138 $m^2$/V.s and n = 1.711; (iii) For 10 K, μ = 0.124 $m^2$/V.s and n = 1.671 (as shown in Fig. S4.1) . With the decrease of temperature, the mobility of the free carriers and the exponent n are increasing, which indicates the dominance of orbital MR term at low temperatures.

**S4.2 Angle dependent TMR at 9T near spin reorientation transition:**

Fig. S4.2 shows the angle dependent transverse magnetoresistance (TMR) at 9 T in close temperature interval near the spin reorientation transition from 120 K to 150 K. We can see the gradual orientation of the spins from ab-plane to the c-axis of the crystal staring from 120 K to 150 K with a drastic change of phase of the MR-θ curve between 140 K and 150 K.

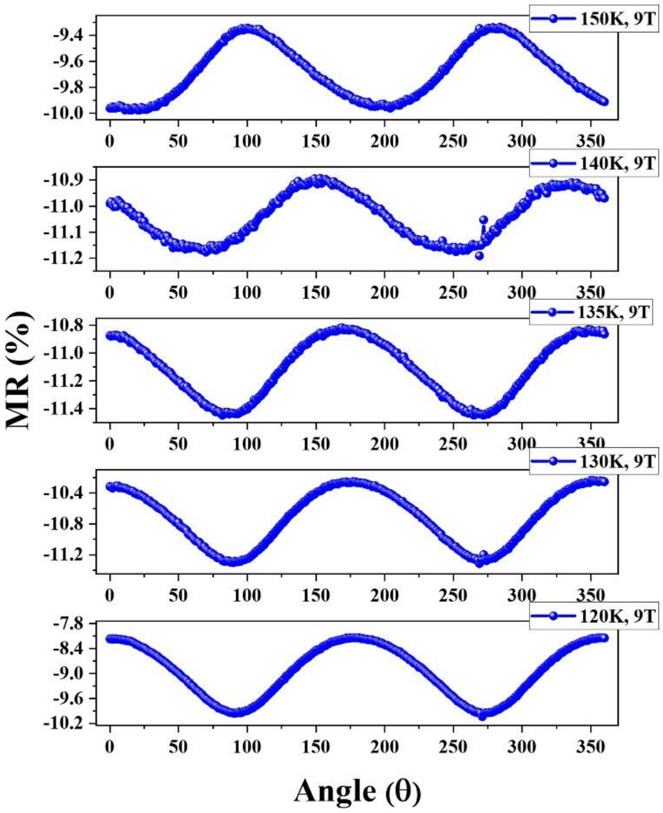


**Figure S4.2** Angle dependent transverse MR at 9 T with the temperature range from 120 K to 150 K, provides a clear indication of spin-reorientation transition in between this temperature range.

## S5. Calculation of AHE from RAW data:

The transverse Hall resistivity ($\rho_{xy}$) of a ferromagnetic material can be described by an empirical formula[3,4] as follows:

$$\rho_{xy} = \rho_{xy}^{OHE} + \rho_{xy}^{AHE} = R_0B + R_SM \quad (1)$$

Here, the first part is the ordinary Hall resistivity ($\rho_{xy}^{OHE}$ = $R_0B$) and the second part is the anomalous Hall resistivity ($\rho_{xy}^{AHE}$ = $R_SM$), $R_0$ and $R_S$ are the ordinary Hall coefficient and anomalous Hall coefficient respectively.

We can obtain the anomalous Hall resistivity ($\rho_{xy}^{AHE}$) from the zero-field intercept by fitting the equation (1) linearly to the magnetic field dependent transverse Hall resistivity ($\rho_{xy}$) curves at higher magnetic field regions (B ≥ 7 T) where $\rho_{xy}$ is linear in magnetic field (B) and the magnetization (M = $M_S$) is saturated. The slope of the linear fit provides the ordinary Hall coefficient ($R_0$) as shown in Fig. S5 (a). Such analysis is valid when the magnetization (M) saturates. From the M-B curves (Fig. 3(a)), we see that M is not saturating above ~ 110 K even after 7 T. Hence, we use the following equation to fit the data,

$$\rho_{xy}/B = R_0 + R_S(M/B) \quad \text{.......................................... (2)}$$

From that fitting of $\rho_{xy}$/B vs M/B at very high field regime (B > 7 T) (like Fig. S5 (b)), we can easily determine the slopes and y-axis intercepts, which provide us the temperature dependent values of $R_S$ and $R_0$ respectively.

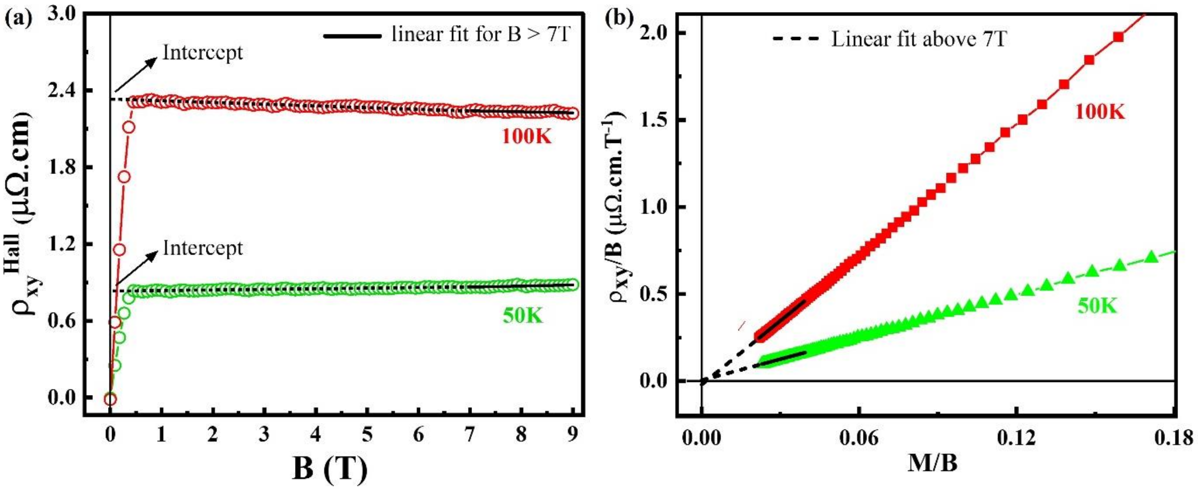


**Figure S5 (a)** $\rho_{xy}^{Hall}$ vs B data for two characteristic temperatures 50 K and 100 K, with a linear fit using Eq. 1 at high fields (B > 7 T). The intercept provides the anomalous Hall contribution. **(b)** Analysis of the same anomalous Hall effect data by using Eq. 2.

## S6. Decoupling different scattering mechanisms of anomalous Hall coefficient $R_S$(T):

Depending on the various scattering mechanisms in ferromagnets, the anomalous Hall resistivity ($\rho_{xy}^{AHE}$) or anomalous Hall coefficient ($R_S$) relates with the longitudinal resistivity ($\rho_{xx}$) by the following scaling relation as:

$$R_S = a\rho_{xx} + b\rho_{xx}^2 \quad \text{....................................... (3)}$$

Here, a and b denote the strengths of the skew-scattering[5,6] and intrinsic[7]/side-jump[8] contributions to the anomalous Hall coefficient, respectively. Both intrinsic and side-jump contributions show $\rho_{xx}^2$ dependence. Being an inherent property of any sample, intrinsic K-L mechanism is almost temperature independent even if $\rho_{xx}$ is temperature dependent, but side-

jump contribution is temperature dependent[9]. The separation between these two mechanisms can be done from the temperature dependence of the $R_S$ vs. T curves by the following procedures[10].

The total longitudinal resistivity ($\rho_{xx}$) can be written as a sum of temperature independent residual resistivity ($\rho_{xx0}$) and temperature dependent part ($\rho_{xxT}$)[11]. So, using ($\rho_{xx0}+\rho_{xxT}$) instead of $\rho_{xx}$ in the scaling relation Eq. (3), the modified scaling equation is:

$$R_S(T) = a(\rho_{xx0}+\rho_{xxT}) + b(\rho_{xx0}+\rho_{xxT})^2 = (a_1\rho_{xx0} + a_2\rho_{xxT}) + (b_1\rho_{xx0}^2 + b_2\rho_{xxT}^2) + c\rho_{xx0}\rho_{xxT} \quad \ldots\ldots..(4)$$

Here, ($a_1\rho_{xx0} + a_2\rho_{xxT}$) is the total skew scattering contribution ($R_S$(SK)), ($b_1\rho_{xx0}^2 + b_2\rho_{xxT}^2$) is the total side-jump scattering or intrinsic K-L contribution ($R_S$(SJ, I)) to the total $R_S$(T). $c\rho_{xx0}\rho_{xxT}$ is the cross term which provides the competition between the different scattering contributions. Also, $a_1 = a_2 = a$, $b_1 = b_2 = b$ and $c = 2b$.

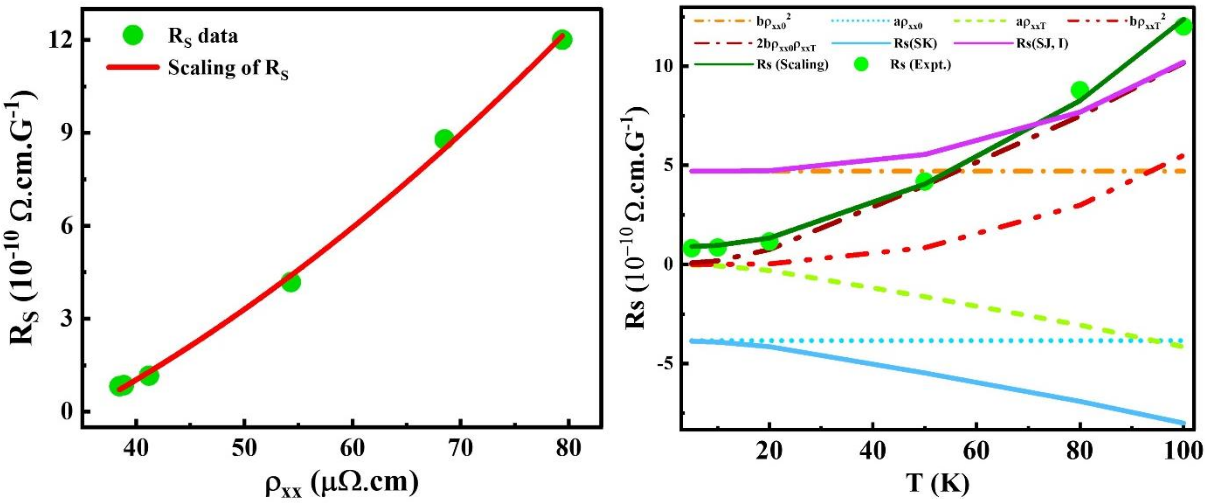


**Figure S6 (a)** Scaling between $R_S$ and $\rho_{xx}$ by the Eq. 3. **(b)** The temperature dependence of anomalous Hall coefficient ($R_S$) is plotted. The individual terms used in Eq. 4, contributing to $R_S$ is plotted with temperature. The temperature dependence of each skew-scattering and side-jump/intrinsic contributions to $R_S$ are plotted via cyan and purple solid line.

Hence, $R_S$ is fitted with Eq. 3 to determine the coefficients a and b. Figure S6 (a) indicates the scaling of Eq. 3 with $\rho_{xx}$, which gives a well agreement with the experimentally determined $R_S$ data. Figure S6 (b) shows the temperature dependence of each contribution associated with $R_S$. Here, $a_1\rho_{xx0}$ and $b_1\rho_{xx0}^2$ terms are temperature independent as shown in Fig. S6 (b). The terms $a_2\rho_{xxT}$, $b_2\rho_{xxT}^2$ and $c\rho_{xx0}\rho_{xxT}$ are dependent on temperature. From the Fig. S6 (b), $a_2\rho_{xxT}$ and $b_2\rho_{xxT}^2$ are acting opposite to each other with the increase of temperature. Here, $b_2\rho_{xxT}^2$ and $c\rho_{xx0}\rho_{xxT}$ are contributing dominantly to the temperature dependent part of $R_S$. Also, the total side-jump mechanism or intrinsic K-L contribution is acting dominantly over skew-scattering mechanism in the experimentally determined value of $R_S$. In association with this, the scaling relation of Eq. 4 provides a well-agreement to the experimentally determined temperature dependent $R_S$ value as indicated by the green solid line in Fig. S6 (b). As intrinsic AHE is weakly temperature dependent[9,12] than the side-jump mechanism and previously it was recognised that electron-magnon scattering can trigger the temperature dependence of side

jump contribution[13]. So, one can conclude that, magnon may be responsible for the side-jump contribution to the AHE in this material.

To confirm this dependency of magnons on the side-jump mechanisms, we have plotted the temperature dependence of extrinsic side jump contribution $R_S^{SJ}$ and the change of resistivity ($\Delta\rho_{xx}$) at high field (9 T) (Fig. 5 main text). We fitted the data in the plotting between $R_S^{SJ}$ and $|\Delta\rho_{xx}|_{9T}$ as shown in the inset of Fig. 5(b). We observe that $R_S^{SJ}$ varies linearly with $|\Delta\rho_{xx}|_{9T}$ within the temperatures 40 K to 120 K, however, deviates below 40 K and above 120 K. This linear behaviour in the temperature range (40 K - 120 K) supports the role of electron-magnon scattering on the AHE via the side-jump mechanism.

## References:


1. Seo, J. *et al.* Nearly room temperature ferromagnetism in a magnetic metal-rich van der Waals metal. *Sci. Adv.* **6**, 1–10 (2020).

2. Mondal, S., Khan, N., Mishra, S. M., Satpati, B. & Mandal, P. Critical behavior in the van der Waals itinerant ferromagnet $Fe_4GeTe_2$. *Phys. Rev. B* **104**, 1–9 (2021).

3. Pugh, E. M. Hall Effect and the Magnetic Properties of Some Ferromagnetic Materials. *Phys. Rev.* **36**, 1503–1511 (1930).

4. Pugh, E. M. & Lippert, T. W. Hall e.m.f. and Intensity of Magnetization. *Phys. Rev.* **42**, 709–713 (1932).

5. Smit, J. The spontaneous hall effect in ferromagnetics I. *Physica* **XXI**, 877–887 (1955).

6. Smit, J. The spontaneous hall effect in ferromagnetics I. *Physica* **24**, 39–51 (1958).

7. Karplus, R. & Luttinger, J. M. Hall effect in ferromagnetics. *Phys. Rev.* **95**, 1154–1160 (1954).

8. Berger, L. Side-jump mechanism for the hall effect of ferromagnets. *Phys. Rev. B* **2**, 4559–4566 (1970).

9. Nagaosa, N., Sinova, J., Onoda, S., MacDonald, A. H. & Ong, N. P. Anomalous Hall effect. *Rev. Mod. Phys.* **82**, 1539–1592 (2010).

10. Jena, R. P., Kumar, D. & Lakhani, A. Scaling analysis of anomalous Hall resistivity in the $Co_2TiAl$ Heusler alloy. *J. Phys. Condens. Matter* **32**, 365703 (2020).

11. Tian, Y., Ye, L. & Jin, X. Proper scaling of the anomalous hall effect. *Phys. Rev. Lett.* **103**, 1–4 (2009).

12. Miyasato, T. *et al.* Crossover Behavior of the Anomalous Hall Effect and Anomalous Nernst Effect in Itinerant Ferromagnets. *Phys. Rev. Lett.* **99**, 86602 (2007).

13. Yang, S. A., Pan, H., Yao, Y. & Niu, Q. Scattering universality classes of side jump in the anomalous Hall effect. *Phys. Rev. B - Condens. Matter Mater. Phys.* **83**, 1–8 (2011).
